# Supplementary material for: GrainSpace: A Large-scale Dataset for Fine-grained and Domain-adaptive Recognition of Cereal Grains
Source: arXiv:2203.05306 source file (2022-03-10)
Supplement: Supplementary file 1 [file appendix.tex]

\section{Appendix}

\begin{figure*}[!htb]
	
	\begin{center}
		\includegraphics[width=\textwidth]{figs/device_appdenix.pdf}
	\end{center}
	\caption{the description and appearance of device.}
	\label{fig:device_appdenix}
\end{figure*}

\begin{figure}[!htb]
	\begin{center}
		\includegraphics[width=0.4\textwidth]{figs/data_distribution_map.png}
	\end{center}
	\caption{The map of the world.}
	\label{fig:grainspace-map}
\end{figure}

\begin{table*}[!htb]
	\centering
	\caption{Detailed performances of R50 \cite{resnet}, DCL \cite{dcl} and Swin Transformer \cite{SwinTrans} on wheat data: different regions vs different device prototypes.}
	\resizebox{0.84\textwidth}{!}{	
		\begin{tabular}{c|c|c|ccccccc|c}
			\toprule
			Model & Region & Device & Normal & F\&S  & SD    & MY    & BN    & AP    & BP    & Total \\\midrule
			\multirow{9}[0]{*}{R50 \cite{resnet}} & \multirow{3}[0]{*}{$R_{1-14}$} 
			
					& P600  & 99.5\% & 85.2\% & 93.0\% & 93.6\% & 98.5\% & 95.5\% & 92.0\% & 93.9\%  \\
			&       & G600  & 99.0\% & 95.1\% & 69.7\% & 77.0\% & 95.2\% & 70.2\% & 54.7\% & 80.1\% \\
			&       & M600  & 99.5\% & 87.1\% & 86.1\% & 80.1\% & 94.7\% & 78.5\% & 87.2\% & 87.6\% \\\cmidrule{2-11}
			& \multirow{3}[0]{*}{$R_{15-18}$} 
					& P600  & 82.3\% & 35.9\% & 80.0\% & 93.9\% & 98.1\% & 83.4\% & 86.4\% & 80.0\% \\
			&       & G600  & 75.7\% & 25.9\% & 73.5\% & 96.4\% & 97.7\% & 89.8\% & 76.7\% & 76.5\% \\
			&       & M600  & 96.8\% & 41.4\% & 95.8\% & 94.5\% & 92.8\% & 47.4\% & 89.2\% & 79.7\% \\\cmidrule{2-11}
			& \multirow{3}[0]{*}{$R_{19-22}$} 
					& P600  & 86.7\% & 34.1\% & 78.2\% & 40.0\% & 96.2\% & 76.8\% & 78.9\% & 70.1\% \\
			&       & G600  & 84.0\% & 38.4\% & 81.6\% & 65.0\% & 96.5\% & 94.3\% & 72.7\% & 76.1\% \\
			&       & M600  & 96.7\% & 56.6\% & 82.8\% & 60.4\% & 85.9\% & 62.8\% & 87.4\% & 76.1\% \\ \midrule
			\multirow{9}[0]{*}{DCL \cite{dcl}} & \multirow{3}[0]{*}{$R_{1-14}$} 
					& P600  & 99.4\% & 83.0\% & 92.1\% & 93.0\% & 97.7\% & 92.0\% & 90.6\% & 92.5\% \\
			&       & G600  & 97.6\% & 80.0\% & 23.3\% & 45.8\% & 39.4\% & 36.6\% & 33.2\% & 50.8\% \\
			&       & M600  & 96.1\% & 0.0\% & 0.0\% & 0.0\% & 0.0\% & 0.0\% & 0.0\% & 13.7\% \\\cmidrule{2-11}
			& \multirow{3}[0]{*}{$R_{15-18}$} 
					& P600  & 72.7\% & 19.1\% & 71.3\% & 83.2\% & 93.5\% & 24.1\% & 69.6\% & 61.9\% \\
			&       & G600  & 75.7\% & 42.2\% & 66.1\% & 91.0\% & 96.5\% & 84.4\% & 74.8\% & 75.8\% \\
			&       & M600  & 96.2\% & 53.4\% & 93.6\% & 93.8\% & 87.7\% & 25.7\% & 82.5\% & 76.1\% \\\cmidrule{2-11}
			& \multirow{3}[0]{*}{$R_{19-22}$} 
					& P600  & 83.2\% & 35.1\% & 66.1\% & 0.0\% & 82.3\% & 44.6\% & 78.5\% & 55.7\% \\
			&       & G600  & 82.2\% & 23.7\% & 79.2\% & 57.9\% & 86.7\% & 92.5\% & 70.2\% & 70.3\% \\
			&       & M600  & 94.7\% & 44.0\% & 75.5\% & 48.0\% & 57.3\% & 42.7\% & 88.0\% & 64.3\% \\\midrule
			\multirow{9}[0]{*}{SwinT \cite{SwinTrans}} & \multirow{3}[0]{*}{$R_{1-14}$} 
					& P600  & 97.4\% & 43.2\% & 20.7\% & 81.2\% & 87.5\% & 25.9\% & 40.0\% & 56.6\% \\
			&       & G600  & 97.0\% & 41.6\% & 17.3\% & 22.6\% & 71.2\% & 0.3\% & 24.5\% & 39.2\% \\
			&       & M600  & 98.8\% & 66.3\% & 52.3\% & 33.5\% & 79.8\% & 41.7\% & 75.9\% & 64.0\% \\\cmidrule{2-11}
			& \multirow{3}[0]{*}{$R_{15-18}$} 
					& P600  & 65.0\% & 0.0\% & 54.1\% & 75.3\% & 94.1\% & 0.0\% & 59.9\% & 49.8\% \\
			&       & G600  & 65.1\% & 0.0\% & 50.0\% & 85.2\% & 92.3\% & 66.2\% & 50.8\% & 58.5\% \\
			&       & M600  & 90.0\% & 0.0\% & 69.9\% & 51.1\% & 63.0\% & 0.0\% & 33.3\% & 43.9\% \\\cmidrule{2-11}
			& \multirow{3}[0]{*}{$R_{19-22}$} 
					& P600  & 76.2\% & 0.0\% & 64.1\% & 0.0\% & 92.8\% & 13.2\% & 61.6\% & 44.0\% \\
			&       & G600  & 74.6\% & 0.0\% & 69.6\% & 31.0\% & 90.8\% & 43.9\% & 49.3\% & 51.3\% \\
			&       & M600  & 93.5\% & 35.1\% & 64.8\% & 20.0\% & 71.7\% & 10.4\% & 78.5\% & 53.4\% \\\bottomrule	
		\end{tabular}

		\label{tab:tab:details_result_wheat_multmodel_region_deivces}
		
	}
\end{table*}

% Please add the following required packages to your document preamble:
% \usepackage{multirow}
\begin{table*}[h]
	\centering
	\caption{ Detailed Performances of R50 \cite{resnet} on wheat, corn and rice data with different device prototypes. (\textcolor{red}{-} and \textcolor{blue}{+} mean that Semi-supervised learning (MixMatch \cite{MixMatch} based on R50 \cite{resnet}) is introduced to train models with unlabeled data).}
	\resizebox{0.95\textwidth}{!}{	
		\begin{tabular}{ccccccccccccc}
			\toprule
			\multirow{2}[0]{*}{Species} & \multicolumn{3}{c}{Train set} & \multirow{2}[0]{*}{Test set} & \multirow{2}[0]{*}{Normal} & \multicolumn{6}{c}{Damaged and Unsound grains} & \multirow{2}[0]{*}{Total} \\
				\cmidrule(lr){2-4} \cmidrule(lr){7-12}
			& P600  & G600  & M600  &       &       & F\&S  & SD    & MY    & BN    & AP    & BP    &  \\\midrule
			\multirow{5}[0]{*}{Wheat} & \checkmark     &       &       
			& P600  & 89.4\% \textcolor{blue}{+ 2.8\%} & 67.2\% \textcolor{blue}{+ 0.5\%} & 19.8\% \textcolor{blue}{+ 42.8\%} & 67.1\% \textcolor{blue}{+ 15.6\%} & 94.9\% \textcolor{blue}{+ 0.4\%} & 73.8\% \textcolor{blue}{+ 2.4\%} & 67.6\% \textcolor{blue}{+ 10.9\%} & 68.5\% \textcolor{blue}{+ 10.6\%} \\
			&       & \checkmark     &       
			& G600  & 93.7\% \textcolor{blue}{+ 0.8\%} & 89.9\% \textcolor{red}{- 4.5\%} & 17.0\% \textcolor{blue}{+ 28.3\%} & 59.7\% \textcolor{blue}{+ 4.6\%} & 86.5\% \textcolor{red}{- 0.7\%} & 54.2\% \textcolor{red}{- 0.1\%} & 43.6\% \textcolor{blue}{+ 7.3\%} & 63.5\% \textcolor{blue}{+ 5.1\%}  \\
			&       &       & \checkmark     
			& M600  & 95.1\% \textcolor{blue}{+ 1.7\%} & 62.3\% \textcolor{red}{- 3.4\%} & 32.9\% \textcolor{blue}{+ 36.5\%} & 54.3\% \textcolor{blue}{+ 10.9\%} & 57.6\% \textcolor{blue}{+ 17.7\%} & 48.7\% \textcolor{red}{- 2.5\%} & 65.1\% \textcolor{blue}{+ 14.1\%} & 59.4\% \textcolor{blue}{+ 10.7\%} \\
			&       & \checkmark     & \checkmark  
			& G600   & 93.7\% \textcolor{blue}{+ 0.6\%} & 89.3\% \textcolor{red}{- 7.4\%} & 19.3\% \textcolor{blue}{- 21.3\%} & 62.1\% \textcolor{blue}{+ 3.9\%} & 81.8\% \textcolor{blue}{+ 5.0\%} & 56.8\% \textcolor{red}{- 3.0\%} & 41.1\% \textcolor{blue}{+ 10.9\%} & 63.4\% \textcolor{blue}{+ 4.5\%} \\
			&       & \checkmark     & \checkmark     
			& M600  & 88.1\% \textcolor{blue}{+ 5.3\%} & 0.1\% \textcolor{blue}{+ 27.1\%} & 0.2\% \textcolor{blue}{+ 7.2\%} & 0.1\% \textcolor{blue}{+22.1\%} & 10.4\% \textcolor{blue}{+ 5.1\%} & 0.5\% \textcolor{blue}{+ 11.0\%} & 4.5\% \textcolor{blue}{+ 25.3\%} & 14.8\% \textcolor{blue}{+ 14.7\%} \\\midrule
			\multirow{2}[0]{*}{Species} & \multicolumn{3}{c}{Training set} & \multirow{2}[0]{*}{Testing set} & \multirow{2}[0]{*}{Normal} & \multicolumn{6}{c}{Damaged and Unsound grains} & \multirow{2}[0]{*}{Total} \\
			\cmidrule(lr){2-4} \cmidrule(lr){7-12}
			& P600  & G600  & M600  &       &       & FM  & SD    & MY    & BN    & AP    & HD    &  \\\midrule
			\multirow{5}[0]{*}{Maize} & \checkmark     &       &       
			& P600  & 99.2\% \textcolor{red}{- 1.5\%} & 99.4\% \textcolor{red}{- 2.1\%} & 93.6\% \textcolor{red}{- 5.7\%} & 86.5\% \textcolor{red}{- 2.8\%} & 98.0\% \textcolor{red}{- 1.5\%} & 96.8\% \textcolor{red}{- 1.0\%} & 84.8\% \textcolor{red}{- 4.1\%} & 94.0\% \textcolor{red}{- 2.7\%} \\
			&       & \checkmark     &       
			& G600  & 97.9\% \textcolor{red}{- 1.4\%} & 85.5\% \textcolor{red}{- 2.4\%} & 88.9\% \textcolor{red}{- 1.5\%} & 75.3\% \textcolor{red}{- 6.0\%} & 95.4\% \textcolor{red}{- 0.6\%} & 92.2\% \textcolor{red}{- 3.1\%} & 70.8\% \textcolor{red}{- 0.3\%} & 86.6\% \textcolor{red}{- 2.2\%} \\
			&       &       & \checkmark     
			& M600  & 95.4\% \textcolor{red}{- 1.7\%} & 52.4\% \textcolor{red}{- 8.3\%} & 85.3\% \textcolor{red}{- 24.3\%} & 81.3\% \textcolor{red}{- 4.1\%} & 94.9\% \textcolor{red}{- 1.3\%} & 91.4\% \textcolor{red}{- 0.3\%} & 79.0\% \textcolor{red}{- 4.6\%} & 82.8\% \textcolor{red}{- 6.4\%} \\
			&       & \checkmark     & \checkmark     
			& G600  & 97.7\% \textcolor{red}{- 1.0\%} & 83.2\% \textcolor{red}{- 1.6\%} & 87.5\% \textcolor{red}{- 2.0\%} & 72.7\% \textcolor{red}{- 3.8\%} & 95.7\% \textcolor{red}{- 1.4\%} & 91.7\% \textcolor{red}{- 1.9\%} & 68.4\% \textcolor{blue}{+ 0.6\%} & 85.3\% \textcolor{red}{- 1.6\%} \\
			&       & \checkmark     & \checkmark     
			& M600 & 67.8\% \textcolor{blue}{+ 8.9\%} & 14.4\% \textcolor{blue}{+ 13.1\%} & 27.3\% \textcolor{blue}{+ 28.3\%} & 31.4\% \textcolor{blue}{+ 24.2\%} & 62.2\% \textcolor{blue}{+ 19.3\%} & 31.7\% \textcolor{blue}{+ 33.9\%} & 1.6\% \textcolor{blue}{+ 42.8\%} & 33.8\% \textcolor{blue}{+ 24.3\%} \\\bottomrule
		\end{tabular}%
	}

	\resizebox{0.95\textwidth}{!}{	
    \begin{tabular}{cccccccccccccc}
    	\toprule
		\multirow{2}[0]{*}{Species} & \multicolumn{3}{c}{Training set} & \multirow{2}[0]{*}{Testing set} & \multicolumn{8}{c}{Categories of Rice Grains}                 & \multirow{2}[0]{*}{Total} \\
			\cmidrule(lr){2-4} \cmidrule(lr){6-13}
		& P600  & G600  & M600  &       & Malis & SQ    & 545   & HF    & WC    & HN    & JZ    & SY    &  \\\midrule
		\multirow{5}[0]{*}{Rice} & \checkmark     &       &       
										 & P600  & 99.2\% & 97.4\% & 98.9\% & 99.0\% & 99.9\% & 99.4\% & 99.7\% & 99.8\% & 99.2\% \\
		&       & \checkmark     &       & G600  & 99.4\% & 95.6\% & 97.8\% & 99.4\% & 99.7\% & 99.5\% & 99.6\% & 99.8\% & 98.9\% \\
		&       &       & \checkmark     & M600  & 93.4\% & 80.0\% & 88.2\% & 91.6\% & 98.0\% & 97.1\% & 98.6\% & 96.8\% & 93.0\% \\
		&       & \checkmark     & \checkmark     & G600  & 99.3\% & 95.0\% & 97.5\% & 99.4\% & 99.7\% & 99.4\% & 99.6\% & 99.8\% & 98.7\% \\
		&       & \checkmark     & \checkmark     & M600  & 4.3\% & 30.0\% & 19.8\% & 21.7\% & 43.5\% & 23.0\% & 46.6\% & 25.7\% & 26.8\%  \\ \bottomrule
	\end{tabular}%

}
	\label{tab:details_result_train_test_deivces}
\end{table*}

\begin{figure*}[!htb]
	
	\begin{center}
		\includegraphics[width=0.8\textwidth]{figs/CAM-visulation.png}
	\end{center}
	\caption{CAM-based results.}
	\label{fig:cam_r}
\end{figure*}

\begin{table*}[]
	\centering
	\caption{Performances of self-supervised learning (MoCo \cite{moco} based on R50 \cite{resnet}) on wheat, corn and rice data with different device prototypes.}
	\resizebox{0.95\textwidth}{!}{
		    \begin{tabular}{cccccccccccccc}
		    \toprule
			\multirow{2}[0]{*}{Species} & \multicolumn{3}{c}{Training set} & \multirow{2}[0]{*}{Testing set} & \multirow{2}[0]{*}{Proportion} & \multirow{2}[0]{*}{Normal} & \multicolumn{6}{c}{Damaged and Unsound Grains} & \multirow{2}[0]{*}{Total} \\
			\cmidrule(lr){2-4} 			\cmidrule(lr){8-13}
			& P600  & G600  & M600  &       &       &       & F\&S  & SD    & MY    & BN    & AP    & BP    &  \\ \midrule
			\multirow{12}[0]{*}{Wheat} 
			& \checkmark &       &       & \multirow{3}[0]{*}{P600} 
												 & 1\%   & 89.7\% & 19.0\% & 60.3\% & 69.5\% & 96.1\% & 27.6\% & 39.8\% & 57.4\% \\
			& \checkmark &       &       &       & 10\%  & 90.2\% & 35.2\% & 59.8\% & 76.3\% & 96.3\% & 22.9\% & 39.2\% & 60.0\% \\
			& \checkmark &       &       &       & 100\% & 89.8\% & 27.4\% & 55.6\% & 72.1\% & 96.1\% & 21.2\% & 34.6\% & 56.7\% \\ \cmidrule(lr){2-14}
			&       & \checkmark &       & \multirow{3}[0]{*}{G600} 
												 & 1\%   & 94.1\% & 59.2\% & 50.4\% & 75.4\% & 94.8\% & 55.6\% & 27.8\% & 65.3\% \\
			&       & \checkmark &       &       & 10\%  & 93.8\% & 51.2\% & 44.5\% & 75.4\% & 95.5\% & 57.0\% & 26.2\% & 63.4\% \\
			&       & \checkmark &       &       & 100\% & 93.7\% & 53.5\% & 40.7\% & 72.2\% & 95.4\% & 49.1\% & 28.4\% & 61.9\% \\ \cmidrule(lr){2-14}
			&       &       & \checkmark & \multirow{3}[0]{*}{M600} 
												 & 1\%   & 94.7\% & 28.0\% & 0.0\% & 20.4\% & 70.1\% & 0.6\% & 7.2\% & 31.6\% \\
			&       &       & \checkmark &       & 10\%  & 95.3\% & 52.0\% & 29.7\% & 21.2\% & 83.2\% & 25.9\% & 12.2\% & 45.6\% \\
			&       &       & \checkmark &       & 100\% & 95.5\% & 51.0\% & 37.2\% & 32.6\% & 82.7\% & 12.0\% & 7.4\% & 45.5\% \\ \cmidrule(lr){2-14}
			
			&       & \checkmark & \checkmark & \multirow{3}{*}[-2.5em]{{\begin{tabular}{c} G600 \\ \textcolor{blue}{M600} \end{tabular}}} 
			& 1\%   & 
			{\begin{tabular}{c} 93.2\% \\ \textcolor{blue}{94.5\%} \end{tabular}}  & 
			{\begin{tabular}{c} 52.5\% \\ \textcolor{blue}{32.3\%} \end{tabular}}  & 
			{\begin{tabular}{c} 30.7\% \\ \textcolor{blue}{10.2\%} \end{tabular}}  & 
			{\begin{tabular}{c} 73.1\% \\ \textcolor{blue}{33.7\%} \end{tabular}}  & 
			{\begin{tabular}{c} 94.7\% \\ \textcolor{blue}{73.8\%} \end{tabular}}  & 
			{\begin{tabular}{c} 37.7\% \\ \textcolor{blue}{9.8\%} \end{tabular}}  & 
			{\begin{tabular}{c} 25.7\% \\ \textcolor{blue}{6.8\%} \end{tabular}}  &
			{\begin{tabular}{c} 58.2\% \\ \textcolor{blue}{37.3\%} \end{tabular}}  \\ \cmidrule(lr){6-14}
			&       & \checkmark & \checkmark &       
			& 10\%  & 
			{\begin{tabular}{c} 93.4\% \\ \textcolor{blue}{94.7\%} \end{tabular}}  & 
			{\begin{tabular}{c} 47.8\% \\ \textcolor{blue}{38.9\%} \end{tabular}}  & 
			{\begin{tabular}{c} 34.8\% \\ \textcolor{blue}{15.2\%} \end{tabular}}  & 
			{\begin{tabular}{c} 74.4\% \\ \textcolor{blue}{36.0\%} \end{tabular}}  & 
			{\begin{tabular}{c} 95.2\% \\ \textcolor{blue}{77.0\%} \end{tabular}}  & 
			{\begin{tabular}{c} 48.8\% \\ \textcolor{blue}{16.1\%} \end{tabular}}  & 
			{\begin{tabular}{c} 26.9\% \\ \textcolor{blue}{9.5\%} \end{tabular}}  & 
			{\begin{tabular}{c} 60.2\% \\ \textcolor{blue}{41.1\%} \end{tabular}}  \\ \cmidrule(lr){6-14}
			&       & \checkmark & \checkmark &       
			& 100\% & 
			{\begin{tabular}{c} 93.3\% \\ \textcolor{blue}{94.5\%} \end{tabular}}  &
			{\begin{tabular}{c} 49.1\% \\ \textcolor{blue}{36.3\%} \end{tabular}}  & 
			{\begin{tabular}{c} 31.7\% \\ \textcolor{blue}{9.2\%} \end{tabular}}  & 
			{\begin{tabular}{c} 73.0\% \\ \textcolor{blue}{31.5\%} \end{tabular}}  & 
			{\begin{tabular}{c} 95.1\% \\ \textcolor{blue}{76.5\%} \end{tabular}}  & 
			{\begin{tabular}{c} 48.1\% \\ \textcolor{blue}{11.9\%} \end{tabular}}  & 
			{\begin{tabular}{c} 26.9\% \\ \textcolor{blue}{10.8\%} \end{tabular}}  & 
			{\begin{tabular}{c} 59.6\% \\ \textcolor{blue}{38.7\%} \end{tabular}}  \\ \bottomrule
			
			\toprule
			\multirow{2}[0]{*}{Species} & \multicolumn{3}{c}{Training set} & \multirow{2}[0]{*}{Testing set} & \multirow{2}[0]{*}{Proportion} & \multirow{2}[0]{*}{Normal} & \multicolumn{6}{c}{Damaged and Unsound Grains} & \multirow{2}[0]{*}{Total} \\
			\cmidrule(lr){2-4} 			\cmidrule(lr){8-13}
			& P600  & G600  & M600  &       &       &       & FM  & SD    & MY    & BN    & AP    & HD    &  \\ \midrule
			\multirow{12}[0]{*}{Maize} 
			& \checkmark &       &       & \multirow{3}[0]{*}{P600} 
												 & 1\%   & 64.1\% & 0.1\% & 0.1\% & 0.1\% & 56.1\% & 0.1\% & 0.1\% & 17.2\% \\
			& \checkmark &       &       &       & 10\%  & 83.4\% & 77.9\% & 0.1\% & 31.8\% & 88.1\% & 49.9\% & 37.8\% & 52.7\% \\
			& \checkmark &       &       &       & 100\% & 86.5\% & 92.8\% & 55.0\% & 59.4\% & 92.6\% & 61.9\% & 58.3\% & 72.4\%  \\ \cmidrule(lr){2-14}
			&       & \checkmark &       & \multirow{3}[0]{*}{G600} 
												 & 1\%   & 0.1\% & 39.3\% & 0.1\% & 0.1\% & 31.1\% & 0.1\% & 15.8\% & 12.3\% \\
			&       & \checkmark &       &       & 10\%  & 80.9\% & 59.7\% & 39.2\% & 44.5\% & 76.3\% & 33.8\% & 32.6\% & 52.4\% \\
			&       & \checkmark &       &       & 100\% & 86.5\% & 64.8\% & 53.3\% & 50.9\% & 84.2\% & 54.0\% & 39.7\% & 61.9\% \\ \cmidrule(lr){2-14}
			&       &       & \checkmark & \multirow{3}[0]{*}{M600} 
												 & 1\%   & 48.2\% & 0.1\% & 0.1\% & 0.1\% & 0.1\% & 0.1\% & 0.1\% & 6.9\% \\
			&       &       & \checkmark &       & 10\%  & 67.1\% & 0.1\% & 0.1\% & 0.1\% & 0.1\% & 6.2\% & 0.1\% & 10.5\% \\
			&       &       & \checkmark &       & 100\% & 74.5\% & 14.0\% & 29.9\% & 53.1\% & 69.2\% & 28.4\% & 1.7\% & 38.7\% \\ \cmidrule(lr){2-14}
			&       & \checkmark & \checkmark & \multirow{3}{*}[-2.5em]{{\begin{tabular}{c} G600 \\ \textcolor{blue}{M600} \end{tabular}}} 
		& 1\%   & 
		{\begin{tabular}{c} 78.2\% \\ \textcolor{blue}{48.6\%} \end{tabular}}  & 
		{\begin{tabular}{c} 0.1\% \\ \textcolor{blue}{0.1\%} \end{tabular}}  & 
		{\begin{tabular}{c} 0.1\% \\ \textcolor{blue}{0.1\%} \end{tabular}}  & 
		{\begin{tabular}{c} 29.9\% \\ \textcolor{blue}{0.1\%} \end{tabular}}  & 
		{\begin{tabular}{c} 3.0\% \\ \textcolor{blue}{0.1\%} \end{tabular}}  & 
		{\begin{tabular}{c} 0.1\% \\ \textcolor{blue}{0.1\%} \end{tabular}}  & 
		{\begin{tabular}{c} 22.3\% \\ \textcolor{blue}{19.6\%} \end{tabular}}  &
		{\begin{tabular}{c} 19.1\% \\ \textcolor{blue}{9.6\%} \end{tabular}}  \\ \cmidrule(lr){6-14}
		&       & \checkmark & \checkmark &       
		& 10\%  & 
		{\begin{tabular}{c} 79.5\% \\ \textcolor{blue}{76.0\%} \end{tabular}}  & 
		{\begin{tabular}{c} 60.6\% \\ \textcolor{blue}{26.1\%} \end{tabular}}  & 
		{\begin{tabular}{c} 40.9\% \\ \textcolor{blue}{4.9\%} \end{tabular}}  & 
		{\begin{tabular}{c} 44.6\% \\ \textcolor{blue}{56.9\%} \end{tabular}}  & 
		{\begin{tabular}{c} 79.6\% \\ \textcolor{blue}{77.4\%} \end{tabular}}  & 
		{\begin{tabular}{c} 40.7\% \\ \textcolor{blue}{39.4\%} \end{tabular}}  & 
		{\begin{tabular}{c} 34.2\% \\ \textcolor{blue}{28.1\%} \end{tabular}}  & 
		{\begin{tabular}{c} 54.3\% \\ \textcolor{blue}{44.1\%} \end{tabular}}  \\ \cmidrule(lr){6-14}
		&       & \checkmark & \checkmark &       
		& 100\% & 
		{\begin{tabular}{c} 87.0\% \\ \textcolor{blue}{80.2\%} \end{tabular}}  &
		{\begin{tabular}{c} 65.1\% \\ \textcolor{blue}{34.3\%} \end{tabular}}  & 
		{\begin{tabular}{c} 54.8\% \\ \textcolor{blue}{38.3\%} \end{tabular}}  & 
		{\begin{tabular}{c} 51.1\% \\ \textcolor{blue}{49.2\%} \end{tabular}}  & 
		{\begin{tabular}{c} 85.3\% \\ \textcolor{blue}{78.9\%} \end{tabular}}  & 
		{\begin{tabular}{c} 53.2\% \\ \textcolor{blue}{48.7\%} \end{tabular}}  & 
		{\begin{tabular}{c} 42.8\% \\ \textcolor{blue}{29.5\%} \end{tabular}}  & 
		{\begin{tabular}{c} 62.8\% \\ \textcolor{blue}{51.3\%} \end{tabular}}  \\ \bottomrule
			
		\end{tabular}%
	}

	\resizebox{0.95\textwidth}{!}{	
	\begin{tabular}{ccccccccccccccc}
		\toprule
		\multirow{2}[0]{*}{Species} & \multicolumn{3}{c}{Training set} & \multirow{2}[0]{*}{Testing set} & \multirow{2}[0]{*}{Proportion} & \multicolumn{8}{c}{Categories of Rice Grains}                 & \multirow{2}[0]{*}{Total} \\
		\cmidrule(lr){2-4} 			\cmidrule(lr){7-14}
		& P600  & G600  & M600  &       &       & Malis & SQ & 545 & HF & WC & HN & JZ & SY &  \\ \midrule
		\multirow{12}[0]{*}{Rice} 
		& \checkmark &       &       & \multirow{3}[0]{*}{P600} 
											 & 1\%   & 11.1\% & 11.1\% & 11.1\% & 11.1\% & 11.1\% & 11.1\% & 11.1\% & 11.1\% & 11.1\% \\
		& \checkmark &       &       &       & 10\%  & 11.1\% & 11.1\% & 11.1\% & 11.1\% & 11.1\% & 11.1\% & 11.1\% & 11.1\% & 11.1\% \\
		& \checkmark &       &       &       & 100\% & 11.1\% & 11.1\% & 11.1\% & 11.1\% & 11.1\% & 11.1\% & 11.1\% & 11.1\% & 11.1\% \\ \cmidrule(lr){2-15}
		&       & \checkmark &       & \multirow{3}[0]{*}{G600} 
										     & 1\%   & 11.1\% & 11.1\% & 11.1\% & 11.1\% & 11.1\% & 11.1\% & 11.1\% & 11.1\% & 11.1\% \\
		&       & \checkmark &       &       & 10\%  & 11.1\% & 11.1\% & 11.1\% & 11.1\% & 11.1\% & 11.1\% & 11.1\% & 11.1\% & 11.1\% \\
		&       & \checkmark &       &       & 100\% & 11.1\% & 11.1\% & 11.1\% & 11.1\% & 11.1\% & 11.1\% & 11.1\% & 11.1\% & 11.1\% \\  \cmidrule(lr){2-15}
		&       &       & \checkmark & \multirow{3}[0]{*}{M600} 
											 & 1\%   & 11.1\% & 11.1\% & 11.1\% & 11.1\% & 11.1\% & 11.1\% & 11.1\% & 11.1\% & 11.1\% \\
		&       &       & \checkmark &       & 10\%  & 11.1\% & 11.1\% & 11.1\% & 11.1\% & 11.1\% & 11.1\% & 11.1\% & 11.1\% & 11.1\% \\
		&       &       & \checkmark &       & 100\% & 11.1\% & 11.1\% & 11.1\% & 11.1\% & 11.1\% & 11.1\% & 11.1\% & 11.1\% & 11.1\% \\ \cmidrule(lr){2-15}

			&       & \checkmark & \checkmark & \multirow{3}{*}[-2.5em]{{\begin{tabular}{c} G600 \\ \textcolor{blue}{M600} \end{tabular}}} 
		& 1\%   & 
		{\begin{tabular}{c} 11.1\% \\ \textcolor{blue}{11.1\%} \end{tabular}}  & 
		{\begin{tabular}{c} 11.1\% \\ \textcolor{blue}{11.1\%} \end{tabular}}  & 
		{\begin{tabular}{c} 11.1\% \\ \textcolor{blue}{11.1\%} \end{tabular}}  & 
		{\begin{tabular}{c} 11.1\% \\ \textcolor{blue}{11.1\%} \end{tabular}}  & 
		{\begin{tabular}{c} 11.1\% \\ \textcolor{blue}{11.1\%} \end{tabular}}  & 
		{\begin{tabular}{c} 11.1\% \\ \textcolor{blue}{11.1\%} \end{tabular}}  & 
		{\begin{tabular}{c} 11.1\% \\ \textcolor{blue}{11.1\%} \end{tabular}}  &
		{\begin{tabular}{c} 11.1\% \\ \textcolor{blue}{11.1\%} \end{tabular}}  &
		{\begin{tabular}{c} 11.1\% \\ \textcolor{blue}{11.1\%} \end{tabular}}  \\ \cmidrule(lr){6-15}
		&       & \checkmark & \checkmark &       
		& 10\%  & 
		{\begin{tabular}{c} 11.1\% \\ \textcolor{blue}{11.1\%} \end{tabular}}  & 
		{\begin{tabular}{c} 11.1\% \\ \textcolor{blue}{11.1\%} \end{tabular}}  & 
		{\begin{tabular}{c} 11.1\% \\ \textcolor{blue}{11.1\%} \end{tabular}}  & 
		{\begin{tabular}{c} 11.1\% \\ \textcolor{blue}{11.1\%} \end{tabular}}  & 
		{\begin{tabular}{c} 11.1\% \\ \textcolor{blue}{11.1\%} \end{tabular}}  & 
		{\begin{tabular}{c} 11.1\% \\ \textcolor{blue}{11.1\%} \end{tabular}}  & 
		{\begin{tabular}{c} 11.1\% \\ \textcolor{blue}{11.1\%} \end{tabular}}  & 
		{\begin{tabular}{c} 11.1\% \\ \textcolor{blue}{11.1\%} \end{tabular}}  & 
		{\begin{tabular}{c} 11.1\% \\ \textcolor{blue}{11.1\%} \end{tabular}}  \\ \cmidrule(lr){6-15}
		&       & \checkmark & \checkmark &       
		& 100\% & 
		{\begin{tabular}{c} 11.1\% \\ \textcolor{blue}{11.1\%} \end{tabular}}  &
		{\begin{tabular}{c} 11.1\% \\ \textcolor{blue}{11.1\%} \end{tabular}}  & 
		{\begin{tabular}{c} 11.1\% \\ \textcolor{blue}{11.1\%} \end{tabular}}  & 
		{\begin{tabular}{c} 11.1\% \\ \textcolor{blue}{11.1\%} \end{tabular}}  & 
		{\begin{tabular}{c} 11.1\% \\ \textcolor{blue}{11.1\%} \end{tabular}}  & 
		{\begin{tabular}{c} 11.1\% \\ \textcolor{blue}{11.1\%} \end{tabular}}  & 
		{\begin{tabular}{c} 11.1\% \\ \textcolor{blue}{11.1\%} \end{tabular}}  & 
		{\begin{tabular}{c} 11.1\% \\ \textcolor{blue}{11.1\%} \end{tabular}}  & 
		{\begin{tabular}{c} 11.1\% \\ \textcolor{blue}{11.1\%} \end{tabular}}  \\ \bottomrule
	\end{tabular}%
	}
\end{table*}

\begin{table*}[h]
	\centering
	\caption{Detailed performances of domain adaptation methods (CDAN \cite{DCAN}, MCD\cite{MCD} and MCC \cite{MCC}) vs. different regions of wheat data (we evaluate P600 and a combination of G600+M600).}
	\resizebox{0.9\textwidth}{!}{		
		\begin{tabular}{ccccccccccc}
			\toprule
			Source $\rightarrow$ Target & Device & Method & Normal & F\&S  & SD    & MY    & BN    & AP    & BP    & Total \\ \midrule
			\multirow{8}[0]{*}{$R_{1-14}\rightarrow R_{15-18}$} & \multirow{4}[0]{*}{P600} & Source only & 11.1\% & 11.1\% & 11.1\% & 11.1\% & 11.1\% & 11.1\% & 11.1\% & 11.1\% \\ \cmidrule(lr){3-11}
			&       & CDAN \cite{DCAN} & 11.1\% & 11.1\% & 11.1\% & 11.1\% & 11.1\% & 11.1\% & 11.1\% & 11.1\% \\
			&       & MCD \cite{MCD}   & 11.1\% & 11.1\% & 11.1\% & 11.1\% & 11.1\% & 11.1\% & 11.1\% & 11.1\% \\
			&       & MCC \cite{MCC}   & 11.1\% & 11.1\% & 11.1\% & 11.1\% & 11.1\% & 11.1\% & 11.1\% & 11.1\% \\ \cmidrule(lr){2-11}
			& \multirow{4}[0]{*}{G600+M600} & Source only & 11.1\% & 11.1\% & 11.1\% & 11.1\% & 11.1\% & 11.1\% & 11.1\% & 11.1\% \\ \cmidrule(lr){3-11}
			&       & CDAN \cite{DCAN}  & 11.1\% & 11.1\% & 11.1\% & 11.1\% & 11.1\% & 11.1\% & 11.1\% & 11.1\% \\
			&       & MCD \cite{MCD}   & 11.1\% & 11.1\% & 11.1\% & 11.1\% & 11.1\% & 11.1\% & 11.1\% & 11.1\% \\
			&       & MCC \cite{MCC}   & 11.1\% & 11.1\% & 11.1\% & 11.1\% & 11.1\% & 11.1\% & 11.1\% & 11.1\% \\ \midrule
			\multirow{8}[0]{*}{$R_{15-18}\rightarrow R_{1-14}$} & \multirow{4}[0]{*}{P600} & Source only & 11.1\% & 11.1\% & 11.1\% & 11.1\% & 11.1\% & 11.1\% & 11.1\% & 11.1\% \\ \cmidrule(lr){3-11}
			&       & CDAN \cite{DCAN}  & 11.1\% & 11.1\% & 11.1\% & 11.1\% & 11.1\% & 11.1\% & 11.1\% & 11.1\% \\
			&       & MCD \cite{MCD}   & 11.1\% & 11.1\% & 11.1\% & 11.1\% & 11.1\% & 11.1\% & 11.1\% & 11.1\% \\
			&       & MCC \cite{MCC}   & 11.1\% & 11.1\% & 11.1\% & 11.1\% & 11.1\% & 11.1\% & 11.1\% & 11.1\% \\ \cmidrule(lr){2-11}
			& \multirow{4}[0]{*}{G600+M600} & Source only & 11.1\% & 11.1\% & 11.1\% & 11.1\% & 11.1\% & 11.1\% & 11.1\% & 11.1\% \\ \cmidrule(lr){3-11}
			&       & CDAN \cite{DCAN}  & 11.1\% & 11.1\% & 11.1\% & 11.1\% & 11.1\% & 11.1\% & 11.1\% & 11.1\% \\
			&       & MCD \cite{MCD}   & 11.1\% & 11.1\% & 11.1\% & 11.1\% & 11.1\% & 11.1\% & 11.1\% & 11.1\% \\
			&       & MCC \cite{MCC}   & 11.1\% & 11.1\% & 11.1\% & 11.1\% & 11.1\% & 11.1\% & 11.1\% & 11.1\% \\ \midrule
			\multirow{8}[0]{*}{$R_{15-18}\rightarrow R_{19-22}$} & \multirow{4}[0]{*}{P600} & Source only & 11.1\% & 11.1\% & 11.1\% & 11.1\% & 11.1\% & 11.1\% & 11.1\% & 11.1\% \\ \cmidrule(lr){3-11}
			&       & CDAN \cite{DCAN}  & 11.1\% & 11.1\% & 11.1\% & 11.1\% & 11.1\% & 11.1\% & 11.1\% & 11.1\% \\
			&       & MCD \cite{MCD}   & 11.1\% & 11.1\% & 11.1\% & 11.1\% & 11.1\% & 11.1\% & 11.1\% & 11.1\% \\
			&       & MCC \cite{MCC}   & 11.1\% & 11.1\% & 11.1\% & 11.1\% & 11.1\% & 11.1\% & 11.1\% & 11.1\% \\ \cmidrule(lr){2-11}
			& \multirow{4}[0]{*}{G600+M600} & Source only & 11.1\% & 11.1\% & 11.1\% & 11.1\% & 11.1\% & 11.1\% & 11.1\% & 11.1\% \\ \cmidrule(lr){3-11}
			&       & CDAN \cite{DCAN}  & 11.1\% & 11.1\% & 11.1\% & 11.1\% & 11.1\% & 11.1\% & 11.1\% & 11.1\% \\
			&       & MCD \cite{MCD}   & 11.1\% & 11.1\% & 11.1\% & 11.1\% & 11.1\% & 11.1\% & 11.1\% & 11.1\% \\
			&       & MCC \cite{MCC}   & 11.1\% & 11.1\% & 11.1\% & 11.1\% & 11.1\% & 11.1\% & 11.1\% & 11.1\% \\ \midrule
			\multirow{8}[0]{*}{$R_{19-22}\rightarrow R_{15-18}$} & \multirow{4}[0]{*}{P600} & Source only & 11.1\% & 11.1\% & 11.1\% & 11.1\% & 11.1\% & 11.1\% & 11.1\% & 11.1\% \\ \cmidrule(lr){3-11}
			&       & CDAN \cite{DCAN}  & 11.1\% & 11.1\% & 11.1\% & 11.1\% & 11.1\% & 11.1\% & 11.1\% & 11.1\% \\
			&       & MCD \cite{MCD}   & 11.1\% & 11.1\% & 11.1\% & 11.1\% & 11.1\% & 11.1\% & 11.1\% & 11.1\% \\
			&       & MCC \cite{MCC}   & 11.1\% & 11.1\% & 11.1\% & 11.1\% & 11.1\% & 11.1\% & 11.1\% & 11.1\% \\ \cmidrule(lr){2-11}
			& \multirow{4}[0]{*}{G600+M600} & Source only & 11.1\% & 11.1\% & 11.1\% & 11.1\% & 11.1\% & 11.1\% & 11.1\% & 11.1\% \\ \cmidrule(lr){3-11}
			&       & CDAN \cite{DCAN}  & 11.1\% & 11.1\% & 11.1\% & 11.1\% & 11.1\% & 11.1\% & 11.1\% & 11.1\% \\
			&       & MCD \cite{MCD}   & 11.1\% & 11.1\% & 11.1\% & 11.1\% & 11.1\% & 11.1\% & 11.1\% & 11.1\% \\
			&       & MCC \cite{MCC}   & 11.1\% & 11.1\% & 11.1\% & 11.1\% & 11.1\% & 11.1\% & 11.1\% & 11.1\% \\ \midrule
			\multirow{8}[0]{*}{$R_{19-22}\rightarrow R_{1-14}$} & \multirow{4}[0]{*}{P600} & Source only & 11.1\% & 11.1\% & 11.1\% & 11.1\% & 11.1\% & 11.1\% & 11.1\% & 11.1\% \\ \cmidrule(lr){3-11}
			&       & CDAN \cite{DCAN}  & 11.1\% & 11.1\% & 11.1\% & 11.1\% & 11.1\% & 11.1\% & 11.1\% & 11.1\% \\
			&       & MCD \cite{MCD}   & 11.1\% & 11.1\% & 11.1\% & 11.1\% & 11.1\% & 11.1\% & 11.1\% & 11.1\% \\
			&       & MCC \cite{MCC}   & 11.1\% & 11.1\% & 11.1\% & 11.1\% & 11.1\% & 11.1\% & 11.1\% & 11.1\% \\ \cmidrule(lr){2-11}
			& \multirow{4}[0]{*}{G600+M600} & Source only & 11.1\% & 11.1\% & 11.1\% & 11.1\% & 11.1\% & 11.1\% & 11.1\% & 11.1\% \\ \cmidrule(lr){3-11}
			&       & CDAN \cite{DCAN}  & 11.1\% & 11.1\% & 11.1\% & 11.1\% & 11.1\% & 11.1\% & 11.1\% & 11.1\% \\
			&       & MCD \cite{MCD}   & 11.1\% & 11.1\% & 11.1\% & 11.1\% & 11.1\% & 11.1\% & 11.1\% & 11.1\% \\
			&       & MCC \cite{MCC}   & 11.1\% & 11.1\% & 11.1\% & 11.1\% & 11.1\% & 11.1\% & 11.1\% & 11.1\% \\ \midrule
			\multirow{8}[0]{*}{$R_{1-14}\rightarrow R_{19-22}$} & \multirow{4}[0]{*}{P600} & Source only & 11.1\% & 11.1\% & 11.1\% & 11.1\% & 11.1\% & 11.1\% & 11.1\% & 11.1\% \\ \cmidrule(lr){3-11}
			&       & CDAN \cite{DCAN}  & 11.1\% & 11.1\% & 11.1\% & 11.1\% & 11.1\% & 11.1\% & 11.1\% & 11.1\% \\
			&       & MCD \cite{MCD}   & 11.1\% & 11.1\% & 11.1\% & 11.1\% & 11.1\% & 11.1\% & 11.1\% & 11.1\% \\
			&       & MCC \cite{MCC}   & 11.1\% & 11.1\% & 11.1\% & 11.1\% & 11.1\% & 11.1\% & 11.1\% & 11.1\% \\ \cmidrule(lr){2-11}
			& \multirow{4}[0]{*}{G600+M600} & Source only & 11.1\% & 11.1\% & 11.1\% & 11.1\% & 11.1\% & 11.1\% & 11.1\% & 11.1\% \\ \cmidrule(lr){3-11}
			&       & CDAN \cite{DCAN}  & 11.1\% & 11.1\% & 11.1\% & 11.1\% & 11.1\% & 11.1\% & 11.1\% & 11.1\% \\
			&       & MCD \cite{MCD}   & 11.1\% & 11.1\% & 11.1\% & 11.1\% & 11.1\% & 11.1\% & 11.1\% & 11.1\% \\
			&       & MCC \cite{MCC}   & 11.1\% & 11.1\% & 11.1\% & 11.1\% & 11.1\% & 11.1\% & 11.1\% & 11.1\% \\ \bottomrule
		\end{tabular}%	
	}
	\label{tab:details_result_domain_regions}
\end{table*}

\begin{table*}[h]
	\centering
	\caption{Detailed performances domain adaptation methods (CDAN \cite{DCAN}, MCD\cite{MCD} and MCC \cite{MCC}) vs. different device prototypes on wheat and maize data.}
	\resizebox{0.8\textwidth}{!}{	
    \begin{tabular}{c|cccccccccc}
    		\toprule
			Species & Source$\rightarrow$Target & Method & Normal & F\&S  & SD    & MY    & BN    & AP    & BP    & Total \\ \midrule
			\multirow{24}[0]{*}{Wheat} & \multirow{4}[0]{*}{P600$\rightarrow$G600} & Source only & 11.1\% & 11.1\% & 11.1\% & 11.1\% & 11.1\% & 11.1\% & 11.1\% & 11.1\% \\ \cmidrule(lr){3-11}
			& & CDAN \cite{DCAN}  & 11.1\% & 11.1\% & 11.1\% & 11.1\% & 11.1\% & 11.1\% & 11.1\% & 11.1\% \\
			& & MCD \cite{MCD}   & 11.1\% & 11.1\% & 11.1\% & 11.1\% & 11.1\% & 11.1\% & 11.1\% & 11.1\% \\
			& & MCC \cite{MCC}   & 11.1\% & 11.1\% & 11.1\% & 11.1\% & 11.1\% & 11.1\% & 11.1\% & 11.1\% \\ \cmidrule(lr){2-11}
			& \multirow{4}[0]{*}{G600$\rightarrow$P600} & Source only & 11.1\% & 11.1\% & 11.1\% & 11.1\% & 11.1\% & 11.1\% & 11.1\% & 11.1\% \\  \cmidrule(lr){3-11}
			& & CDAN \cite{DCAN} & 11.1\% & 11.1\% & 11.1\% & 11.1\% & 11.1\% & 11.1\% & 11.1\% & 11.1\% \\
			& & MCD \cite{MCD}   & 11.1\% & 11.1\% & 11.1\% & 11.1\% & 11.1\% & 11.1\% & 11.1\% & 11.1\% \\
			& & MCC \cite{MCC}   & 11.1\% & 11.1\% & 11.1\% & 11.1\% & 11.1\% & 11.1\% & 11.1\% & 11.1\% \\ \cmidrule(lr){2-11}
			& \multirow{4}[0]{*}{G600$\rightarrow$M600} & Source only & 11.1\% & 11.1\% & 11.1\% & 11.1\% & 11.1\% & 11.1\% & 11.1\% & 11.1\% \\  \cmidrule(lr){3-11}
			& & CDAN \cite{DCAN}  & 11.1\% & 11.1\% & 11.1\% & 11.1\% & 11.1\% & 11.1\% & 11.1\% & 11.1\% \\
			& & MCD \cite{MCD}   & 11.1\% & 11.1\% & 11.1\% & 11.1\% & 11.1\% & 11.1\% & 11.1\% & 11.1\% \\
			& & MCC \cite{MCC}   & 11.1\% & 11.1\% & 11.1\% & 11.1\% & 11.1\% & 11.1\% & 11.1\% & 11.1\% \\ \cmidrule(lr){2-11}
			& \multirow{4}[0]{*}{M600$\rightarrow$G600} & Source only & 11.1\% & 11.1\% & 11.1\% & 11.1\% & 11.1\% & 11.1\% & 11.1\% & 11.1\% \\  \cmidrule(lr){3-11}
			& & CDAN \cite{DCAN}  & 11.1\% & 11.1\% & 11.1\% & 11.1\% & 11.1\% & 11.1\% & 11.1\% & 11.1\% \\
			& & MCD \cite{MCD}   & 11.1\% & 11.1\% & 11.1\% & 11.1\% & 11.1\% & 11.1\% & 11.1\% & 11.1\% \\
			& & MCC \cite{MCC}   & 11.1\% & 11.1\% & 11.1\% & 11.1\% & 11.1\% & 11.1\% & 11.1\% & 11.1\% \\ \cmidrule(lr){2-11}
			& \multirow{4}[0]{*}{M600$\rightarrow$P600} & Source only & 11.1\% & 11.1\% & 11.1\% & 11.1\% & 11.1\% & 11.1\% & 11.1\% & 11.1\% \\  \cmidrule(lr){3-11}
			& & CDAN \cite{DCAN}  & 11.1\% & 11.1\% & 11.1\% & 11.1\% & 11.1\% & 11.1\% & 11.1\% & 11.1\% \\
			& & MCD \cite{MCD}   & 11.1\% & 11.1\% & 11.1\% & 11.1\% & 11.1\% & 11.1\% & 11.1\% & 11.1\% \\
			& & MCC \cite{MCC}   & 11.1\% & 11.1\% & 11.1\% & 11.1\% & 11.1\% & 11.1\% & 11.1\% & 11.1\% \\ \cmidrule(lr){2-11}
			& \multirow{4}[0]{*}{P600$\rightarrow$M600} & Source only & 11.1\% & 11.1\% & 11.1\% & 11.1\% & 11.1\% & 11.1\% & 11.1\% & 11.1\% \\  \cmidrule(lr){3-11}
			& & CDAN \cite{DCAN}  & 11.1\% & 11.1\% & 11.1\% & 11.1\% & 11.1\% & 11.1\% & 11.1\% & 11.1\% \\
			& & MCD \cite{MCD}   & 11.1\% & 11.1\% & 11.1\% & 11.1\% & 11.1\% & 11.1\% & 11.1\% & 11.1\% \\
			& & MCC \cite{MCC}   & 11.1\% & 11.1\% & 11.1\% & 11.1\% & 11.1\% & 11.1\% & 11.1\% & 11.1\% \\ \bottomrule
			\toprule
			Species & Source$\rightarrow$Target & Method & Normal & FM  & SD    & MY    & BN    & AP    & HD   & Total \\ \midrule
			\multirow{24}[0]{*}{Maize} & \multirow{4}[0]{*}{P600$\rightarrow$G600} & Source only & 11.1\% & 11.1\% & 11.1\% & 11.1\% & 11.1\% & 11.1\% & 11.1\% & 11.1\% \\ \cmidrule(lr){3-11}
			& & CDAN \cite{DCAN}  & 11.1\% & 11.1\% & 11.1\% & 11.1\% & 11.1\% & 11.1\% & 11.1\% & 11.1\% \\
			& & MCD \cite{MCD}   & 11.1\% & 11.1\% & 11.1\% & 11.1\% & 11.1\% & 11.1\% & 11.1\% & 11.1\% \\
			& & MCC \cite{MCC}   & 11.1\% & 11.1\% & 11.1\% & 11.1\% & 11.1\% & 11.1\% & 11.1\% & 11.1\% \\ \cmidrule(lr){2-11}
			& \multirow{4}[0]{*}{G600$\rightarrow$P600} & Source only & 11.1\% & 11.1\% & 11.1\% & 11.1\% & 11.1\% & 11.1\% & 11.1\% & 11.1\% \\  \cmidrule(lr){3-11}
			& & CDAN \cite{DCAN} & 11.1\% & 11.1\% & 11.1\% & 11.1\% & 11.1\% & 11.1\% & 11.1\% & 11.1\% \\
			& & MCD \cite{MCD}   & 11.1\% & 11.1\% & 11.1\% & 11.1\% & 11.1\% & 11.1\% & 11.1\% & 11.1\% \\
			& & MCC \cite{MCC}   & 11.1\% & 11.1\% & 11.1\% & 11.1\% & 11.1\% & 11.1\% & 11.1\% & 11.1\% \\ \cmidrule(lr){2-11}
			& \multirow{4}[0]{*}{G600$\rightarrow$M600} & Source only & 11.1\% & 11.1\% & 11.1\% & 11.1\% & 11.1\% & 11.1\% & 11.1\% & 11.1\% \\  \cmidrule(lr){3-11}
			& & CDAN \cite{DCAN}  & 11.1\% & 11.1\% & 11.1\% & 11.1\% & 11.1\% & 11.1\% & 11.1\% & 11.1\% \\
			& & MCD \cite{MCD}   & 11.1\% & 11.1\% & 11.1\% & 11.1\% & 11.1\% & 11.1\% & 11.1\% & 11.1\% \\
			& & MCC \cite{MCC}   & 11.1\% & 11.1\% & 11.1\% & 11.1\% & 11.1\% & 11.1\% & 11.1\% & 11.1\% \\ \cmidrule(lr){2-11}
			& \multirow{4}[0]{*}{M600$\rightarrow$G600} & Source only & 11.1\% & 11.1\% & 11.1\% & 11.1\% & 11.1\% & 11.1\% & 11.1\% & 11.1\% \\  \cmidrule(lr){3-11}
			& & CDAN \cite{DCAN}  & 11.1\% & 11.1\% & 11.1\% & 11.1\% & 11.1\% & 11.1\% & 11.1\% & 11.1\% \\
			& & MCD \cite{MCD}   & 11.1\% & 11.1\% & 11.1\% & 11.1\% & 11.1\% & 11.1\% & 11.1\% & 11.1\% \\
			& & MCC \cite{MCC}   & 11.1\% & 11.1\% & 11.1\% & 11.1\% & 11.1\% & 11.1\% & 11.1\% & 11.1\% \\ \cmidrule(lr){2-11}
			& \multirow{4}[0]{*}{M600$\rightarrow$P600} & Source only & 11.1\% & 11.1\% & 11.1\% & 11.1\% & 11.1\% & 11.1\% & 11.1\% & 11.1\% \\  \cmidrule(lr){3-11}
			& & CDAN \cite{DCAN}  & 11.1\% & 11.1\% & 11.1\% & 11.1\% & 11.1\% & 11.1\% & 11.1\% & 11.1\% \\
			& & MCD \cite{MCD}   & 11.1\% & 11.1\% & 11.1\% & 11.1\% & 11.1\% & 11.1\% & 11.1\% & 11.1\% \\
			& & MCC \cite{MCC}   & 11.1\% & 11.1\% & 11.1\% & 11.1\% & 11.1\% & 11.1\% & 11.1\% & 11.1\% \\ \cmidrule(lr){2-11}
			& \multirow{4}[0]{*}{P600$\rightarrow$M600} & Source only & 11.1\% & 11.1\% & 11.1\% & 11.1\% & 11.1\% & 11.1\% & 11.1\% & 11.1\% \\  \cmidrule(lr){3-11}
			& & CDAN \cite{DCAN}  & 11.1\% & 11.1\% & 11.1\% & 11.1\% & 11.1\% & 11.1\% & 11.1\% & 11.1\% \\
			& & MCD \cite{MCD}   & 11.1\% & 11.1\% & 11.1\% & 11.1\% & 11.1\% & 11.1\% & 11.1\% & 11.1\% \\
			& & MCC \cite{MCC}   & 11.1\% & 11.1\% & 11.1\% & 11.1\% & 11.1\% & 11.1\% & 11.1\% & 11.1\% \\ \bottomrule
					
	\end{tabular}%
		
	}
	\label{tab:details_result_domain_devices_wheatandmaize}
\end{table*}

\begin{table*}[h]
	\centering
	\caption{Detailed performances domain adaptation methods (CDAN \cite{DCAN}, MCD\cite{MCD} and MCC \cite{MCC}) vs. different device prototypes on rice data.}
	\resizebox{0.9\textwidth}{!}{		
		\begin{tabular}{ccccccccccc}
			\toprule
			Source $\rightarrow$ Target & Method & Mails & SQ    & 545   & HF    & WC    & HN    & HZ    & SY    & Total \\ \midrule
			\multirow{4}[0]{*}{P600$\rightarrow$G600} & Source only & 11.1\% & 11.1\% & 11.1\% & 11.1\% & 11.1\% & 11.1\% & 11.1\% & 11.1\% & 11.1\% \\ \cmidrule(lr){2-11}
			& CDAN \cite{DCAN}  & 11.1\% & 11.1\% & 11.1\% & 11.1\% & 11.1\% & 11.1\% & 11.1\% & 11.1\% & 11.1\% \\
			& MCD \cite{MCD}   & 11.1\% & 11.1\% & 11.1\% & 11.1\% & 11.1\% & 11.1\% & 11.1\% & 11.1\% & 11.1\% \\
			& MCC \cite{MCC}  & 11.1\% & 11.1\% & 11.1\% & 11.1\% & 11.1\% & 11.1\% & 11.1\% & 11.1\% & 11.1\% \\ \midrule
			\multirow{4}[0]{*}{G600$\rightarrow$P600} & Source only & 11.1\% & 11.1\% & 11.1\% & 11.1\% & 11.1\% & 11.1\% & 11.1\% & 11.1\% & 11.1\% \\ \cmidrule(lr){2-11}
			& CDAN \cite{DCAN}  & 11.1\% & 11.1\% & 11.1\% & 11.1\% & 11.1\% & 11.1\% & 11.1\% & 11.1\% & 11.1\% \\
			& MCD \cite{MCD}   & 11.1\% & 11.1\% & 11.1\% & 11.1\% & 11.1\% & 11.1\% & 11.1\% & 11.1\% & 11.1\% \\
			& MCC \cite{MCC}   & 11.1\% & 11.1\% & 11.1\% & 11.1\% & 11.1\% & 11.1\% & 11.1\% & 11.1\% & 11.1\% \\ \midrule
			\multirow{4}[0]{*}{G600$\rightarrow$M600} & Source only & 11.1\% & 11.1\% & 11.1\% & 11.1\% & 11.1\% & 11.1\% & 11.1\% & 11.1\% & 11.1\% \\ \cmidrule(lr){2-11}
			& CDAN \cite{DCAN}  & 11.1\% & 11.1\% & 11.1\% & 11.1\% & 11.1\% & 11.1\% & 11.1\% & 11.1\% & 11.1\% \\
			& MCD \cite{MCD}   & 11.1\% & 11.1\% & 11.1\% & 11.1\% & 11.1\% & 11.1\% & 11.1\% & 11.1\% & 11.1\% \\
			& MCC \cite{MCC}   & 11.1\% & 11.1\% & 11.1\% & 11.1\% & 11.1\% & 11.1\% & 11.1\% & 11.1\% & 11.1\% \\ \midrule
			\multirow{4}[0]{*}{M600$\rightarrow$G600} & Source only & 11.1\% & 11.1\% & 11.1\% & 11.1\% & 11.1\% & 11.1\% & 11.1\% & 11.1\% & 11.1\% \\ \cmidrule(lr){2-11}
			& CDAN \cite{DCAN}  & 11.1\% & 11.1\% & 11.1\% & 11.1\% & 11.1\% & 11.1\% & 11.1\% & 11.1\% & 11.1\% \\
			& MCD \cite{MCD}   & 11.1\% & 11.1\% & 11.1\% & 11.1\% & 11.1\% & 11.1\% & 11.1\% & 11.1\% & 11.1\% \\
			& MCC \cite{MCC}   & 11.1\% & 11.1\% & 11.1\% & 11.1\% & 11.1\% & 11.1\% & 11.1\% & 11.1\% & 11.1\% \\ \midrule
			\multirow{4}[0]{*}{M600$\rightarrow$P600} & Source only & 11.1\% & 11.1\% & 11.1\% & 11.1\% & 11.1\% & 11.1\% & 11.1\% & 11.1\% & 11.1\% \\ \cmidrule(lr){2-11}
			& CDAN \cite{DCAN}  & 11.1\% & 11.1\% & 11.1\% & 11.1\% & 11.1\% & 11.1\% & 11.1\% & 11.1\% & 11.1\% \\
			& MCD \cite{MCD}   & 11.1\% & 11.1\% & 11.1\% & 11.1\% & 11.1\% & 11.1\% & 11.1\% & 11.1\% & 11.1\% \\
			& MCC \cite{MCC}   & 11.1\% & 11.1\% & 11.1\% & 11.1\% & 11.1\% & 11.1\% & 11.1\% & 11.1\% & 11.1\% \\ \midrule
			\multirow{4}[0]{*}{P600$\rightarrow$M600} & Source only & 11.1\% & 11.1\% & 11.1\% & 11.1\% & 11.1\% & 11.1\% & 11.1\% & 11.1\% & 11.1\% \\ \cmidrule(lr){2-11}
			& CDAN \cite{DCAN}  & 11.1\% & 11.1\% & 11.1\% & 11.1\% & 11.1\% & 11.1\% & 11.1\% & 11.1\% & 11.1\% \\
			& MCD \cite{MCD}   & 11.1\% & 11.1\% & 11.1\% & 11.1\% & 11.1\% & 11.1\% & 11.1\% & 11.1\% & 11.1\% \\
			& MCC \cite{MCC}   & 11.1\% & 11.1\% & 11.1\% & 11.1\% & 11.1\% & 11.1\% & 11.1\% & 11.1\% & 11.1\% \\ \bottomrule
		\end{tabular}%	
	}
	\label{tab:details_result_domain_devices_rice}
\end{table*}

\begin{figure*}[!htb]
	
	\begin{center}
		\includegraphics[width=0.8\textwidth]{figs/ssl_fig.png}
	\end{center}
	\caption{Using self-supervised learning, different proportion of label data can bring the performances. based on R50 with MOCO.}
	\label{fig:ssl_p}
\end{figure*}
